# Supplementary material for: GenSys: A Scalable Fixed-point Engine for Maximal Controller Synthesis over Infinite State Spaces
Source: arXiv:2107.08794 source file (2021-08-16)
Supplement: Supplementary file 1 [file appendix.tex]

\section{Appendix Informal}

\subsection{Safety Algorithm}
\label{safety-algorithm}
The algorithm representing the greatest fixed-point equation in Section \ref{ssec:fixedp-engine} in Algorithm \ref{alg: safety}.

\begin{algorithm}
\SetAlgoLined
\SetKwInOut{Input}{Input}
\SetKwInOut{Output}{Output}
\Input{ Game formulation \wpr, which includes the safe region $G$}
\Output{ Winning region $X$,  if algorithm terminates}
 $X$ := True \;
 $W$ := $Proj(\wpr(X))$ \;
 \While{$(X \wedge G) \nRightarrow (W \wedge G)$}{
  $X$ := $W$\;
  $W$ := $Proj(\wpr(X))$
 }
 return $(X \wedge G)$;
 \caption{Safety fixed-point}
 \label{alg: safety}
\end{algorithm}

Algorithm \ref{alg: safety} takes the game formulation as input and returns the winning region for the controller,  if it terminates. The winning region is a quantifier free formula in the base theory.  $Proj$ is the projection operation that we use to project quantifiers from the game formulation at every step in the algorithm,  to return an equivalent quantifier free formula.

\subsection{Proof Sketch - Non Lattice:}

\DD{The $X_i$ s you compute are the set of states from which the controller can play safely for at least "i" moves.

When $X_{k+1} = X_k$,  from any state in $X_k$ the controller has a way of playing safe forever.}

\emph{Soundness:} We claim that if the algorithm terminates, then it returns the winning region for the controller.  It is sufficient to show that the set of states $X \wedge G$ of the algorithm at every step is safe.  We can show this by induction.  In the first step i.e.,  the base case,  $X \wedge G$ is safe due to the conjunction with $G$.  According to the formulation in section \ref{ssec:game-formulation},  $WP$ represents the \textbf{exact} set of states from where the controller can take the system into the safe region after which all moves the environment also ensures the system staying within the safe region. This combined step move is a single step for the algorithm.  Since $W$ computed in iteration $i-1$ is assigned to $X$ in iteration $i$,  it suffices to reason about $X \wedge G$.  In general $X_i \wedge G$ computed after step $i$ denotes the \textbf{exact} set of \textbf{safe} states for which the system stays in $G$ for \textbf{at least} $i$ steps.  Thus,  if the algorithm terminates at some step $k$ (i.e.,  $X_{k-1} \wedge G = X_k \wedge G$), then it implies that the controller has a way to ensure that the system stays in the safe region forever.

\DD{If the controller has a way of winning (ie. playing safe forever)  from a state "s", then clearly "s" must belong to $X_k$.}

Assume not.  Then there exists a state $s$ which was missed.  This is not possible due to the fact that at every step,  the formulation in Section \ref{ssec:game-formulation} computes the weakest set of states for the controller to stay in the safe region,  against any move of the environment.

\DD{Follows that $X_k$ is the exact set of winning states.}

The procedure may not terminate due to the state space being infinite.

\subsection{Proof Sketch:}
\emph{Background:} 
We consider an \textbf{abstract lattice $A$} over quantifier free predicate logic formulae,  for a given theory.  In this lattice,  disjunction represents join operation and logical implication denotes ordering i.e.,  an element B is "higher up" in the lattice than element A if and only if 'A implies B'  The top element of the lattice is the formula \emph{True} and the bottom element of the lattice is the formula \emph{False}.  Let the free variables in the formulae belong to the set $V$.  
Given a domain $D$,  the state space $S$ is over $D^{|V|}$.  The \textbf{concrete lattice $C$} is over the subsets of $S$ where set union represents the join operation and the subset operation represents ordering. The top element is $S$ whereas the bottom element is the empty set $\phi$. The \textbf{concretization function} $\Gamma$ maps elements of $A$ to elements of $C$ and represents the concrete semantics of a given formula.  Thus, $\Gamma(True) = S$ and $\Gamma(False) = \phi$.  Since the domain can be infinite,  the lattices can have infinite height and width.

\emph{Existence of a Fixed-Point:} The function $\wpr\circ Proj$ is a monotone function of the form $\wpr\circ Proj: A \rightarrow A$ i.e. ,  it takes as input and element of lattice $A$ and returns as output an element of $A$. The intersection operation in $\wpr$ ensures monotonicity and a decreasing sequence.  Since every element of A can be mapped to an element of B which is a complete lattice,  lattice A is also a complete lattice.  By Knaster Tarski theorem,  a fixed-point exists.

\emph{Completeness:}   The algorithm starts with the top element of the lattice $True$ and at every step computes $\wpr\circ Proj$.  Due to the function being monotone, the algorithm will climb down the lattice in $\wpr$.  Since the lattice has infinite height,  the algorithm may never terminate and thus,  is not complete. However,  we have empirically observed that by representing the safe region as a "bounded formula," which is natural,  the algorithm terminates.

\emph{Soundness:} We claim that if the algorithm terminates, then it returns the winning region for the controller.  It is sufficient to show that the set of states $X \wedge G$ of the algorithm at every step is safe.  We can show this by induction.  In the first step i.e.,  the base case,  $X \wedge G$ is safe due to a conjunction with $G$.  According to the formulation in section \ref{ssec:fixedp-engine},  $W$ represents the \textbf{exact} set of states from where the controller can take the system into the safe region after which all moves the environment also ensures the system staying within the safe region. This combined step move is a single step for the algorithm.  Since $W$ computed in iteration $i-1$ is assigned to $X$ in iteration $i$,  it suffices to reason about $X \wedge G$.  In general $X_i \wedge G$ computed after step $i$ denotes the \textbf{exact} set of \textbf{safe} states for which the system stays in $G$ for \textbf{at least} $i$ steps.  

Termination with $False$ at step $i$ denotes that the system can stay in $G$ for at most $i$ steps,  and hence it is not possible to always stay within the safe region and thus no controller exists.  Termination with a satisfiable predicate $X \wedge G$ at step $i$ implies that the region at step $i-1$ and $i$ are equivalent.  Thus,  this region can stay within $G$ always and a controller exists.

The region returned is \textbf{maximal} because at every step,  the weakest set of states is returned.

\emph{AE mode:} The algorithm is exactly same for the case where the environment plays first,  except for the fact that \wpr \ is now:
\subsection{Wolfgang Algorithm for Reachability}

\subsubsection{Game Formulation}
For the Wolfgang approach,  we modify the game formulation as follows.  The property is reachability. We split \wpr \ into \wpr E and \wpr C respectively,  one for each players move.

$$
\begin{array}{lcl}
\wpr C(X)& \equiv & \exists s'. (
Con(s, s') \wedge  (G(s') \vee X(s')))
\end{array}
$$

$$
\begin{array}{lcl}
\wpr E(X)& \equiv & \forall s'. (
Env(s, s') \implies  (G(s') \vee X(s')))
\end{array}
$$

The algorithm representing the least fixed-point equation is Algorithm \ref{alg: wolfgang} which takes the above two game formulations as input and returns the winning regions for the environment ($XE$) and controller ($XC$) respectively,  if it terminates. The winning regions are quantifier free formulae in the base theory.  $Proj$ is defined as earlier.

The arguments for completeness and maximality remain similar to the argument for Algorithm \ref{alg: safety}, except that we have to now explain it in the case of two separate regions.

\emph{Soundness}: In this algorithm,  instead of computing for a combined move,  we compute for a each player in parallel (although we are still computing the winning region for the controller for both starting players).  Thus, step 0 for the controller is the set of states from where there exists a move such that he reach reach the the goal in one step.  Step 0 for the environment is the set of states from where all moves reach the the goal in one step.
For any step $I$ in the algorithm,  the environment states $WE$ denote the states from where controller can win the game in atmost i steps, when environment starts and the controller states $WC$ denote the states from where controller can win the game in atmost i steps, when controller starts. The termination condition is necessary and sufficient for soundness. The termination condition separately checks validity for the controller and environment states

\subsubsection{Relating the two algorithms}
For a fixed controller, environment and safe region, let Algorithm \ref{alg: safety} with EA formulation return the invariant $XEA$.  Similarly,  for AE, let the algorithm return $XAE$.
We claim that $ \overline{XEA} = XA$ and $ \overline{XAE} = XE$.

The proof sketch is as follows.  $XEA$ is the set of states from where the controller can stay in the safe region no matter what the environment plays, when the controller starts the game.  $ \overline{XEA}$ is the set of states from where the environment can always reach an unsafe state no matter what controller plays,  when controller plays first.  This is nothing but $XA$ where controller is now the environment.

Similarly,  for the other claim.

\begin{algorithm}
\SetAlgoLined
\SetKwInOut{Input}{Input}
\SetKwInOut{Output}{Output}
\Input{ Game formulations \wpr E and \wpr C, which include the reach region $G$}
\Output{ Winning regions $XE$ and $XC$,  if algorithm terminates}
 $XE$ := False \;
 $XC$ := False \;
 $WE$ := $Proj(\wpr E(XC))$ \;
 $WC$ := $Proj(\wpr C(XE))$ \;
 \While{$[(WE \vee G) \nRightarrow (XE \vee G)] \vee [(WC \vee G) \nRightarrow (XC \vee G)]$}{
  $XE$ := $WE$\;
  $XC$ := $WC$\;
  $WE$ := $Proj(\wpr E(XC))$\;
  $WC$ := $Proj(\wpr C(XE))$\;
 }
 return $(XE \vee G), \ (XC \vee G)$;
 \caption{Reachability fixed-point: Wolfgang}
 \label{alg: wolfgang}
\end{algorithm}

\subsection{JSYN-VG Correction}

This section can be used in the preprint version that can be attached along with the tool submission.  Here I plan to explain the correct AE formulation in JSYN-VG, using temporary variables,  for which we compare.
\subsubsection{Starting player:} Depending on who starts first, the game can be modelled as an AE or EA game i.e.  ForAll Exists or Exists ForAll game.  The E player is the controller or protagonist i.e.  Cinderella in our case.  The invariant returned may be different if the starting players are interchanged.  For example,  for our game,  from the state $s =[b1=3, b2=3, b3=0, b4=0, b5=0]$,  Cinderella can always win if she plays first and not if Stepmother plays first.  This is because Cinderella can start by emptying buckets $b1$ and $b2$ whereas Stepmother can overflow them thereby violating the safety specification.  Hence $s$ being part of the final invariant can be dependent on the starting player. 

\emph{Effect of tactic on AA:}
Depending on the game formulation we observed that different tactics give different results.  For example,  if we encode the EA game as an AA game i.e.  we assume that the controller can make non-deterministic moves,  then the formula structure changes.  In such a case,  we observe that even the tactic \verb|qe2| does not scale.  In such a case,  formula simplification becomes necessary and the tactical (combination of tactics) \verb|Then(qe2, simplify)| performs better.  However, the best performing tactic for this setting was \verb|Then(qe2_rec, ctx-solver-simplify)|.  This shows the effect of tactics on our approach.  We discuss more in the benchmarks. \Stanly{If not discussed, then remove this line}

It should be noted that ConSynth and JSyn-VG encodes the Cinderella game as a safety game in AE.  SimSynth solves the dual game i.e.  it solves a reachability game for Stepmother where she plays first i.e.  an EA game where Stepmother is the E player.  SimSynth's column shows a successful strategy extraction for both plays whereas the other tools in the table return a controller or unrealizable, which is consistent with GenSys.  GenSys shows the results for both EA and AE.
